# Supplementary material for: Beyond Negative Transfer: Disentangled Preference-Guided Diffusion for Cross-Domain Sequential Recommendation
Source: arXiv:2509.00389 source file (2025-08-30)
Supplement: Supplementary file 1 [file Appendix.tex]

% \begin{table*}[htbp]
%   \centering
%   \caption{Performance comparison across baselines on four cross-domain datasets. \textbf{Bold} indicates the best result, and \underline{underline} marks the second-best. \textbf{Imp. (\%)} denotes the relative improvement of our model over the strongest baseline. * indicates statistical significance over the best baseline under paired t-test with \( p < 0.05 \).}
%   \label{tab:transposed_results}
%   \small
%   \setlength{\tabcolsep}{1mm}
%   \begin{tabular}{ll| rrrr|rrrrrrrrrrr | r}
%     \toprule
%     \textbf{Dataset} & \textbf{Metric} & \textbf{SAS} & \textbf{SRGNN} & \textbf{TCSR} & \textbf{DiffuRec} & \textbf{CGRec} & \textbf{PSJNet} & \textbf{MIFN} & \textbf{C2DSR} & \textbf{PCDSR} & \textbf{EAGCL} & \textbf{LEAGCN} & \textbf{ABXI} & \textbf{C2DREIF} & \textbf{DREAM} & \textbf{Our} & \textbf{Imp. (\%)} \\
%     \midrule
%     \textbf{Movie} & MRR & 3.79 & 3.85 & 3.71 & 5.65 & 4.37 & 4.63 & 5.05 & 5.54 & 5.77 & 5.69 & 5.58 & 5.07 & 6.70 & \underline{8.74} & \textbf{10.95} * & +25.3\% \\
%      & N@5 & 3.23 & 3.27 & 3.71 & 5.96 & 4.46 & 4.06 & 4.41 & 4.76 & 4.93 & 5.13 & 4.15 & 5.29 & 5.80 & \underline{9.52} & \textbf{11.60} * & +21.8\% \\
%      & N@10 & 3.69 & 3.78 & 4.41 & 6.94 & 5.33 & 4.76 & 5.20 & 5.76 & 5.79 & 6.01 & 5.59 & 6.31 & 7.14 & \underline{10.58} & \textbf{13.34} * & +26.1\% \\
%      & H@5 & 3.99 & 4.19 & 5.18 & 8.14 & 5.81 & 5.30 & 5.51 & 6.47 & 6.21 & 6.01 & 6.41 & 7.23 & 7.93 & \underline{13.21} & \textbf{15.68} * & +18.7\% \\
%      & H@10 & 5.20 & 5.81 & 7.36 & 11.17 & 8.54 & 7.53 & 8.29 & 9.55 & 8.89 & 8.20 & 8.67 & 10.41 & 12.08 & \underline{16.49} & \textbf{21.15} * & +28.2\% \\
%     \cmidrule(lr){2-18}
%     \textbf{Book} & MRR & 1.81 & 1.78 & 2.15 & 2.30 & 1.56 & 2.44 & 2.51 & 2.55 & 2.44 & 2.74 & 2.57 & 1.75 & 2.80 & \underline{4.08} & \textbf{4.92} * & +20.5\% \\
%      & N@5 & 1.41 & 1.40 & 2.19 & 2.42 & 1.64 & 2.07 & 2.12 & 2.17 & 2.03 & 2.02 & 2.08 & 1.82 & 2.37 & \underline{4.24} & \textbf{5.16} * & +21.6\% \\
%      & N@10 & 1.71 & 1.66 & 2.50 & 2.89 & 1.94 & 2.35 & 2.31 & 2.45 & 2.31 & 2.30 & 2.26 & 2.18 & 2.71 & \underline{4.87} & \textbf{5.79} * & +18.9\% \\
%      & H@5 & 1.83 & & 2.98 & 3.37 & 2.25 & 2.58 & 2.46 & 2.84 & 2.60 & 2.67 & 2.41 & 2.48 & 3.03 & \underline{5.58} & \textbf{6.67} * & +19.6\% \\
%      & H@10 & 2.75 & & 3.92 & 4.80 & 3.18 & 3.28 & 3.07 & 3.75 & 2.31 & 3.50 & 3.67 & 3.61 & 4.11 & \underline{7.34} & \textbf{8.63} * & +17.5\% \\
%     \midrule
%     \textbf{Food} & MRR & 7.30 & & 7.25 & 7.85 & 8.19 & 8.33 & 8.55 & 8.91 & 9.87 & 9.93 & 9.14 & 9.19 & \underline{10.17} & 10.00 & \textbf{11.20} * & +10.1\% \\
%      & N@5 & 6.90 & & 7.17 & 8.46 & 8.73 & 8.07 & 8.28 & 8.65 & 9.57 & 9.05 & 8.76 & 9.89 & 10.06 & \underline{10.75} & \textbf{12.01} * & +11.7\% \\
%      & N@10 & 7.79 & & 8.26 & 9.13 & 9.43 & 8.77 & 9.01 & 9.71 & 10.72 & 10.22 & 9.85 & 10.50 & 10.93 & \underline{11.74} & \textbf{13.07} * & +11.3\% \\
%      & H@5 & 8.92 & & 9.24 & 11.10 & 11.21 & 10.28 & 10.43 & 11.24 & 12.34 & 12.54 & 12.70 & 12.74 & 12.85 & \underline{14.27} & \textbf{15.75} * & +10.4\% \\
%      & H@10 & 11.68 & & 12.62 & 13.21 & 13.40 & 12.45 & 12.71 & 14.54 & 15.94 & 15.07 & 15.85 & 14.63 & 15.54 & \underline{17.29} & \textbf{19.04} * & +10.1\% \\
% \cmidrule(lr){2-18}
%     \textbf{Kitchen} & MRR & 3.79 & & 4.24 & 3.60 & 3.99 & 4.10 & 4.09 & 4.65 & 4.78 & 4.89 & 4.78 & 4.70 & 4.98 & \underline{5.04} & \textbf{5.56} * & +10.3\% \\
%      & N@5 & 3.35 & & 3.22 & 3.90 & 4.25 & 3.68 & 3.57 & 4.16 & 4.37 & 4.28 & 4.12 & 5.10 & 4.52 & \underline{5.44} & \textbf{6.02} * & +10.7\% \\
%      & N@10 & 3.93 & & 5.66 & 4.55 & 4.86 & 4.32 & 4.29 & 4.94 & 5.08 & 5.16 & 5.28 & 5.75 & 5.31 & \underline{6.37} & \textbf{7.01} * & +10.0\% \\
%      & H@5 & 4.78 & & 4.79 & 5.62 & 5.81 & 5.17 & 4.86 & 5.74 & 6.06 & 6.22 & 6.07 & 7.12 & 6.22 & \underline{7.85} & \textbf{8.65} * & +10.1\% \\
%      & H@10 & 6.62 & & 5.66 & 7.67 & 7.70 & 7.15 & 7.08 & 8.18 & 8.27 & 8.37 & 8.58 & 9.12 & 8.67 & \underline{10.73} & \textbf{11.74} * & +9.4\% \\
%     \midrule
%     \bottomrule
%   \end{tabular}
% \end{table*}
